# Supplementary material for: An Empirical Study of Deep Learning Models for Vulnerability Detection
Source: arXiv:2212.08109 source file (2023-02-12)
Supplement: Supplementary file 1 [file appendix.tex]

\appendices

\section{Code features}

\begin{enumerate}
\item group: \verb|macros|
\begin{itemize}
	\item \verb|preproc_ifdef|
	\item \verb|preproc_if|
	\item \verb|preproc_function_def|
	\item \verb|preproc_arg|
	\item \verb|preproc_params|
	\item \verb|preproc_def|
	\item \verb|preproc_else|
	\item \verb|preproc_defined|
	\item \verb|preproc_call|
	\item \verb|preproc_directive|
	\item \verb|preproc_elif|
\end{itemize}
\item \verb|__asm__|
\item \verb|lexical.num_chars|
\item group: \verb|pointer dereference|
\begin{itemize}
	\item \verb|field_expression|
	\item \verb|pointer_expression|
\end{itemize}
\item group: \verb|array dereference|
\begin{itemize}
	\item \verb|subscript_designator|
	\item \verb|subscript_expression|
\end{itemize}
\item \verb|for_statement|
\item group: \verb|while/do-while|
\begin{itemize}
    \item \verb|while_statement|
    \item \verb|do_statement|
\end{itemize}
\item \verb|call_expression|
\item \verb|if_statement|
\item group: \verb|control-flow jumps|
\begin{itemize}
    \item \verb|break_statement|
    \item \verb|continue_statement|
    \item \verb|return_statement|
\end{itemize}
\item group: \verb|unstructured control-flow|
\begin{itemize}
    \item \verb|labeled_statement|
    \item \verb|goto_statement|
\end{itemize}
\item group: \verb|switch/case|
\begin{itemize}
    \item \verb|switch_statement|
    \item \verb|case_statement|
\end{itemize}
\item \verb|comment|
\end{enumerate}

\section{Big CWE grouping table}
% Please add the following required packages to your document preamble:
% \usepackage{multirow}
\begin{table}[h!]
\centering
\caption{CWE groupings}\label{fig:cwe-grouping}
\begin{tabular}{|l|l|l|}
\hline
CWE Group (example count)                          & CWE ID   & Description                                                                                        \\ \hline
\multirow{5}{*}{Buffer overflow (37291)}           & CWE-119  & Improper Restriction of Operations within the Bounds of a Memory Buffer                            \\ \cline{2-3} 
                                                   & CWE-120  & Buffer Copy without Checking Size of Input ('Classic Buffer Overflow')                             \\ \cline{2-3} 
                                                   & CWE-125  & Out-of-bounds Read                                                                                 \\ \cline{2-3} 
                                                   & CWE-129  & Improper Validation of Array Index                                                                 \\ \cline{2-3} 
                                                   & CWE-787  & Out-of-bounds Write                                                                                \\ \hline
\multirow{19}{*}{Input validation (25514)}         & CWE-134  & Use of Externally-Controlled Format String                                                         \\ \cline{2-3} 
                                                   & CWE-20   & Improper Input Validation                                                                          \\ \cline{2-3} 
                                                   & CWE-22   & Improper Limitation of a Pathname to a Restricted Directory ('Path Traversal')                     \\ \cline{2-3} 
                                                   & CWE-354  & Improper Validation of Integrity Check Value                                                       \\ \cline{2-3} 
                                                   & CWE-426  & Untrusted Search Path                                                                              \\ \cline{2-3} 
                                                   & CWE-494  & Download of Code Without Integrity Check                                                           \\ \cline{2-3} 
                                                   & CWE-502  & Deserialization of Untrusted Data                                                                  \\ \cline{2-3} 
                                                   & CWE-59   & Improper Link Resolution Before File Access ('Link Following')                                     \\ \cline{2-3} 
                                                   & CWE-601  & URL Redirection to Untrusted Site ('Open Redirect')                                                \\ \cline{2-3} 
                                                   & CWE-611  & Improper Restriction of XML External Entity Reference                                              \\ \cline{2-3} 
                                                   & CWE-706  & Use of Incorrectly-Resolved Name or Reference                                                      \\ \cline{2-3} 
                                                   & CWE-74   & Improper Neutralization of Special Elements in Output Used by a Downstream Component ('Injection') \\ \cline{2-3} 
                                                   & CWE-77   & Improper Neutralization of Special Elements used in a Command ('Command Injection')                \\ \cline{2-3} 
                                                   & CWE-78   & Improper Neutralization of Special Elements used in an OS Command ('OS Command Injection')         \\ \cline{2-3} 
                                                   & CWE-79   & Improper Neutralization of Input During Web Page Generation ('Cross-site Scripting')               \\ \cline{2-3} 
                                                   & CWE-89   & Improper Neutralization of Special Elements used in an SQL Command ('SQL Injection')               \\ \cline{2-3} 
                                                   & CWE-90   & Improper Neutralization of Special Elements used in an LDAP Query ('LDAP Injection')               \\ \cline{2-3} 
                                                   & CWE-93   & Improper Neutralization of CRLF Sequences ('CRLF Injection')                                       \\ \cline{2-3} 
                                                   & CWE-94   & Improper Control of Generation of Code ('Code Injection')                                          \\ \hline
\multirow{31}{*}{Privilege escalation (32749)}     & CWE-1021 & Improper Restriction of Rendered UI Layers or Frames                                               \\ \cline{2-3} 
                                                   & CWE-200  & Exposure of Sensitive Information to an Unauthorized Actor                                         \\ \cline{2-3} 
                                                   & CWE-209  & Generation of Error Message Containing Sensitive Information                                       \\ \cline{2-3} 
                                                   & CWE-254  & CWE CATEGORY: 7PK - Security Features                                                              \\ \cline{2-3} 
                                                   & CWE-255  & CWE CATEGORY: Credentials Management Errors                                                        \\ \cline{2-3} 
                                                   & CWE-264  & CWE CATEGORY: Permissions, Privileges, and Access Controls                                         \\ \cline{2-3} 
                                                   & CWE-269  & Improper Privilege Management                                                                      \\ \cline{2-3} 
                                                   & CWE-281  & Improper Preservation of Permissions                                                               \\ \cline{2-3} 
                                                   & CWE-284  & Improper Access Control                                                                            \\ \cline{2-3} 
                                                   & CWE-285  & Improper Authorization                                                                             \\ \cline{2-3} 
                                                   & CWE-287  & Improper Authentication                                                                            \\ \cline{2-3} 
                                                   & CWE-290  & Authentication Bypass by Spoofing                                                                  \\ \cline{2-3} 
                                                   & CWE-295  & Improper Certificate Validation                                                                    \\ \cline{2-3} 
                                                   & CWE-310  & CWE CATEGORY: Cryptographic Issues                                                                 \\ \cline{2-3} 
                                                   & CWE-311  & Missing Encryption of Sensitive Data                                                               \\ \cline{2-3} 
                                                   & CWE-320  & CWE CATEGORY: Key Management Errors                                                                \\ \cline{2-3} 
                                                   & CWE-327  & Use of a Broken or Risky Cryptographic Algorithm                                                   \\ \cline{2-3} 
                                                   & CWE-330  & Use of Insufficiently Random Values                                                                \\ \cline{2-3} 
                                                   & CWE-331  & Insufficient Entropy                                                                               \\ \cline{2-3} 
                                                   & CWE-345  & Insufficient Verification of Data Authenticity                                                     \\ \cline{2-3} 
                                                   & CWE-346  & Origin Validation Error                                                                            \\ \cline{2-3} 
                                                   & CWE-347  & Improper Verification of Cryptographic Signature                                                   \\ \cline{2-3} 
                                                   & CWE-352  & Cross-Site Request Forgery (CSRF)                                                                  \\ \cline{2-3} 
                                                   & CWE-358  & Improperly Implemented Security Check for Standard                                                 \\ \cline{2-3} 
                                                   & CWE-522  & Insufficiently Protected Credentials                                                               \\ \cline{2-3} 
                                                   & CWE-532  & Insertion of Sensitive Information into Log File                                                   \\ \cline{2-3} 
                                                   & CWE-668  & Exposure of Resource to Wrong Sphere                                                               \\ \cline{2-3} 
                                                   & CWE-693  & Protection Mechanism Failure                                                                       \\ \cline{2-3} 
                                                   & CWE-732  & Incorrect Permission Assignment for Critical Resource                                              \\ \cline{2-3} 
                                                   & CWE-862  & Missing Authorization                                                                              \\ \cline{2-3} 
                                                   & CWE-918  & Server-Side Request Forgery (SSRF)                                                                 \\ \hline
\multirow{14}{*}{Resource allocation/free (33748)} & CWE-399  & CWE CATEGORY: Resource Management Errors                                                           \\ \cline{2-3} 
                                                   & CWE-400  & Uncontrolled Resource Consumption                                                                  \\ \cline{2-3} 
                                                   & CWE-404  & Improper Resource Shutdown or Release                                                              \\ \cline{2-3} 
                                                   & CWE-415  & Double Free                                                                                        \\ \cline{2-3} 
                                                   & CWE-416  & Use After Free                                                                                     \\ \cline{2-3} 
                                                   & CWE-476  & NULL Pointer Dereference                                                                           \\ \cline{2-3} 
                                                   & CWE-664  & Improper Control of a Resource Through its Lifetime                                                \\ \cline{2-3} 
                                                   & CWE-665  & Improper Initialization                                                                            \\ \cline{2-3} 
                                                   & CWE-763  & Release of Invalid Pointer or Reference                                                            \\ \cline{2-3} 
                                                   & CWE-769  & DEPRECATED: Uncontrolled File Descriptor Consumption                                               \\ \cline{2-3} 
                                                   & CWE-770  & Allocation of Resources Without Limits or Throttling                                               \\ \cline{2-3} 
                                                   & CWE-772  & Missing Release of Resource after Effective Lifetime                                               \\ \cline{2-3} 
                                                   & CWE-824  & Access of Uninitialized Pointer                                                                    \\ \cline{2-3} 
                                                   & CWE-909  & Missing Initialization of Resource                                                                 \\ \hline
\multirow{12}{*}{Value propagation errors (15126)} & CWE-172  & Encoding Error                                                                                     \\ \cline{2-3} 
                                                   & CWE-189  & CWE CATEGORY: Numeric Errors                                                                       \\ \cline{2-3} 
                                                   & CWE-19   & CWE CATEGORY: Data Processing Errors                                                               \\ \cline{2-3} 
                                                   & CWE-190  & Integer Overflow or Wraparound                                                                     \\ \cline{2-3} 
                                                   & CWE-191  & Integer Underflow (Wrap or Wraparound)                                                             \\ \cline{2-3} 
                                                   & CWE-252  & Unchecked Return Value                                                                             \\ \cline{2-3} 
                                                   & CWE-369  & Divide By Zero                                                                                     \\ \cline{2-3} 
                                                   & CWE-617  & Reachable Assertion                                                                                \\ \cline{2-3} 
                                                   & CWE-674  & Uncontrolled Recursion                                                                             \\ \cline{2-3} 
                                                   & CWE-682  & Incorrect Calculation                                                                              \\ \cline{2-3} 
                                                   & CWE-704  & Incorrect Type Conversion or Cast                                                                  \\ \cline{2-3} 
                                                   & CWE-835  & Loop with Unreachable Exit Condition ('Infinite Loop')                                             \\ \hline
\end{tabular}
\end{table}

\section{Model reproduction}
